# Supplementary material for: Can AI Design a Better nnU-Net? A Hypothesis-Driven Architecture Discovery Loop from Failures to Design Rules
Source: arXiv:2611.32384 source file (2026-11-24)
Supplement: Supplementary file 1 [file xref_supp.tex]

\makeatletter
\expandafter\gdef\csname XS@sec:s_overview\endcsname{S1}
\expandafter\gdef\csname XS@sec:s_overview@cref\endcsname{[section][1][]S1}
\expandafter\gdef\csname XS@sec:s_protocol\endcsname{S2}
\expandafter\gdef\csname XS@sec:s_protocol@cref\endcsname{[section][2][]S2}
\expandafter\gdef\csname XS@sec:s_harness\endcsname{S2.1}
\expandafter\gdef\csname XS@sec:s_harness@cref\endcsname{[subsection][1][2]S2.1}
\expandafter\gdef\csname XS@sec:p-protocol\endcsname{S2.2}
\expandafter\gdef\csname XS@sec:p-protocol@cref\endcsname{[subsection][2][2]S2.2}
\expandafter\gdef\csname XS@sec:p-setting\endcsname{S2.2}
\expandafter\gdef\csname XS@sec:p-setting@cref\endcsname{[subsection][2][2]S2.2}
\expandafter\gdef\csname XS@sec:p-resolution\endcsname{S2.2}
\expandafter\gdef\csname XS@sec:p-resolution@cref\endcsname{[subsection][2][2]S2.2}
\expandafter\gdef\csname XS@sec:s-reading\endcsname{S2.3}
\expandafter\gdef\csname XS@sec:s-reading@cref\endcsname{[subsection][3][2]S2.3}
\expandafter\gdef\csname XS@sec:s-xxnet\endcsname{S3}
\expandafter\gdef\csname XS@sec:s-xxnet@cref\endcsname{[section][3][]S3}
\expandafter\gdef\csname XS@sec:s-archspec\endcsname{S3.1}
\expandafter\gdef\csname XS@sec:s-archspec@cref\endcsname{[subsection][1][3]S3.1}
\expandafter\gdef\csname XS@tab:s-archspec\endcsname{S1}
\expandafter\gdef\csname XS@tab:s-archspec@cref\endcsname{[table][1][]S1}
\expandafter\gdef\csname XS@tab:s-stagecost\endcsname{S2}
\expandafter\gdef\csname XS@tab:s-stagecost@cref\endcsname{[table][2][]S2}
\expandafter\gdef\csname XS@sec:s-stagecost\endcsname{S3.2}
\expandafter\gdef\csname XS@sec:s-stagecost@cref\endcsname{[subsection][2][3]S3.2}
\expandafter\gdef\csname XS@sec:s-erf\endcsname{S3.3}
\expandafter\gdef\csname XS@sec:s-erf@cref\endcsname{[subsection][3][3]S3.3}
\expandafter\gdef\csname XS@sec:s-designation\endcsname{S3.4}
\expandafter\gdef\csname XS@sec:s-designation@cref\endcsname{[subsection][4][3]S3.4}
\expandafter\gdef\csname XS@fig:s-erf\endcsname{S1}
\expandafter\gdef\csname XS@fig:s-erf@cref\endcsname{[figure][1][]S1}
\expandafter\gdef\csname XS@sec:s_base\endcsname{S4}
\expandafter\gdef\csname XS@sec:s_base@cref\endcsname{[section][4][]S4}
\expandafter\gdef\csname XS@sec:s-moved\endcsname{S5}
\expandafter\gdef\csname XS@sec:s-moved@cref\endcsname{[section][5][]S5}
\expandafter\gdef\csname XS@sec:s_team\endcsname{S6}
\expandafter\gdef\csname XS@sec:s_team@cref\endcsname{[section][6][]S6}
\expandafter\gdef\csname XS@tab:s-designation\endcsname{S3}
\expandafter\gdef\csname XS@tab:s-designation@cref\endcsname{[table][3][]S3}
\expandafter\gdef\csname XS@tab:base\endcsname{S4}
\expandafter\gdef\csname XS@tab:base@cref\endcsname{[table][4][]S4}
\expandafter\gdef\csname XS@sec:s_llmuse\endcsname{S6.1}
\expandafter\gdef\csname XS@sec:s_llmuse@cref\endcsname{[subsection][1][6]S6.1}
\expandafter\gdef\csname XS@fig:s-gallery-amos\endcsname{S2}
\expandafter\gdef\csname XS@fig:s-gallery-amos@cref\endcsname{[figure][2][]S2}
\expandafter\gdef\csname XS@tab:s-candidates\endcsname{S5}
\expandafter\gdef\csname XS@tab:s-candidates@cref\endcsname{[table][5][]S5}
\expandafter\gdef\csname XS@fig:s-loop\endcsname{S3}
\expandafter\gdef\csname XS@fig:s-loop@cref\endcsname{[figure][3][]S3}
\expandafter\gdef\csname XS@tab:s-hit\endcsname{S6}
\expandafter\gdef\csname XS@tab:s-hit@cref\endcsname{[table][6][]S6}
\expandafter\gdef\csname XS@fig:s-conv\endcsname{S4}
\expandafter\gdef\csname XS@fig:s-conv@cref\endcsname{[figure][4][]S4}
\expandafter\gdef\csname XS@sec:s_errors\endcsname{S6.2}
\expandafter\gdef\csname XS@sec:s_errors@cref\endcsname{[subsection][2][6]S6.2}
\expandafter\gdef\csname XS@sec:s_stage1\endcsname{S7}
\expandafter\gdef\csname XS@sec:s_stage1@cref\endcsname{[section][7][]S7}
\expandafter\gdef\csname XS@sec:p-carries\endcsname{S8}
\expandafter\gdef\csname XS@sec:p-carries@cref\endcsname{[section][8][]S8}
\expandafter\gdef\csname XS@tab:s-curse\endcsname{S7}
\expandafter\gdef\csname XS@tab:s-curse@cref\endcsname{[table][7][]S7}
\expandafter\gdef\csname XS@tab:s-prov\endcsname{S8}
\expandafter\gdef\csname XS@tab:s-prov@cref\endcsname{[table][8][]S8}
\expandafter\gdef\csname XS@fig:p-traj\endcsname{S5}
\expandafter\gdef\csname XS@fig:p-traj@cref\endcsname{[figure][5][]S5}
\expandafter\gdef\csname XS@tab:llmuse_roles\endcsname{S9}
\expandafter\gdef\csname XS@tab:llmuse_roles@cref\endcsname{[table][9][]S9}
\expandafter\gdef\csname XS@tab:an_process_safeguards\endcsname{S10}
\expandafter\gdef\csname XS@tab:an_process_safeguards@cref\endcsname{[table][10][]S10}
\expandafter\gdef\csname XS@tab:s_stage1_arms\endcsname{S11}
\expandafter\gdef\csname XS@tab:s_stage1_arms@cref\endcsname{[table][11][]S11}
\expandafter\gdef\csname XS@tab:llmuse_calls\endcsname{S11}
\expandafter\gdef\csname XS@tab:llmuse_calls@cref\endcsname{[table][11][]S11}
\expandafter\gdef\csname XS@tab:p-attrib\endcsname{S12}
\expandafter\gdef\csname XS@tab:p-attrib@cref\endcsname{[table][12][]S12}
\expandafter\gdef\csname XS@tab:an_heldout_seeds\endcsname{S13}
\expandafter\gdef\csname XS@tab:an_heldout_seeds@cref\endcsname{[table][13][]S13}
\expandafter\gdef\csname XS@sec:s_heldout\endcsname{S9}
\expandafter\gdef\csname XS@sec:s_heldout@cref\endcsname{[section][9][]S9}
\makeatother
