# Supplementary material for: Can AI Design a Better nnU-Net? A Hypothesis-Driven Architecture Discovery Loop from Failures to Design Rules
Source: arXiv:2611.32384 source file (2026-11-24)
Supplement: Supplementary file 2 [file supp_keys.tex]

% AUTO-GENERATED by paper_v1/supp_keys.py from runs/trials/*/result.json, the candidate specs and the KiTS23 plan -- do not edit by hand
\makeatletter
\expandafter\gdef\csname R@s1.amos.stock.mean\endcsname{87.71}
\expandafter\gdef\csname R@s1.amos.stock.n\endcsname{3}
\expandafter\gdef\csname R@s1.arch.V7A1.dec.gmac\endcsname{118.0}
\expandafter\gdef\csname R@s1.arch.V7A1.dec.gmac_pct\endcsname{35}
\expandafter\gdef\csname R@s1.arch.V7A1.dec.params\endcsname{6.94}
\expandafter\gdef\csname R@s1.arch.V7A1.enc.gmac\endcsname{255.2}
\expandafter\gdef\csname R@s1.arch.V7A1.enc.params\endcsname{24.10}
\expandafter\gdef\csname R@s1.arch.V7A1.gmac\endcsname{373.5}
\expandafter\gdef\csname R@s1.arch.V7A1.params\endcsname{31.04}
\expandafter\gdef\csname R@s1.arch.V7C1.dec.gmac\endcsname{118.0}
\expandafter\gdef\csname R@s1.arch.V7C1.dec.gmac_pct\endcsname{35}
\expandafter\gdef\csname R@s1.arch.V7C1.dec.params\endcsname{6.94}
\expandafter\gdef\csname R@s1.arch.V7C1.enc.gmac\endcsname{138.8}
\expandafter\gdef\csname R@s1.arch.V7C1.enc.params\endcsname{14.17}
\expandafter\gdef\csname R@s1.arch.V7C1.gmac\endcsname{257.0}
\expandafter\gdef\csname R@s1.arch.V7C1.params\endcsname{21.11}
\expandafter\gdef\csname R@s1.arch.base.dec.gmac\endcsname{338.3}
\expandafter\gdef\csname R@s1.arch.base.dec.params\endcsname{17.17}
\expandafter\gdef\csname R@s1.arch.base.enc.gmac\endcsname{138.8}
\expandafter\gdef\csname R@s1.arch.base.enc.params\endcsname{14.03}
\expandafter\gdef\csname R@s1.arch.base.gmac\endcsname{477.3}
\expandafter\gdef\csname R@s1.arch.base.params\endcsname{31.20}
\expandafter\gdef\csname R@s1.fresh.agent.2se\endcsname{11}
\expandafter\gdef\csname R@s1.fresh.agent.n\endcsname{21}
\expandafter\gdef\csname R@s1.fresh.agent.pos\endcsname{19}
\expandafter\gdef\csname R@s1.fresh.n\endcsname{25}
\expandafter\gdef\csname R@s1.fresh.n.2se\endcsname{13}
\expandafter\gdef\csname R@s1.fresh.n.pos\endcsname{23}
\expandafter\gdef\csname R@s1.ho.brats.L1.d\endcsname{\ensuremath{-0.02}}
\expandafter\gdef\csname R@s1.ho.brats.L1.mean\endcsname{82.95}
\expandafter\gdef\csname R@s1.ho.brats.L1.n\endcsname{1}
\expandafter\gdef\csname R@s1.ho.brats.L1.s0\endcsname{82.95}
\expandafter\gdef\csname R@s1.ho.brats.L3.d\endcsname{\ensuremath{+0.07}}
\expandafter\gdef\csname R@s1.ho.brats.L3.mean\endcsname{83.05}
\expandafter\gdef\csname R@s1.ho.brats.L3.n\endcsname{1}
\expandafter\gdef\csname R@s1.ho.brats.L3.s0\endcsname{83.05}
\expandafter\gdef\csname R@s1.ho.brats.V7A1.d\endcsname{\ensuremath{-0.06}}
\expandafter\gdef\csname R@s1.ho.brats.V7A1.mean\endcsname{83.17}
\expandafter\gdef\csname R@s1.ho.brats.V7A1.n\endcsname{3}
\expandafter\gdef\csname R@s1.ho.brats.V7A1.s0\endcsname{83.21}
\expandafter\gdef\csname R@s1.ho.brats.V7A1.s1\endcsname{83.16}
\expandafter\gdef\csname R@s1.ho.brats.V7A1.s2\endcsname{83.15}
\expandafter\gdef\csname R@s1.ho.brats.V7C1.d\endcsname{\ensuremath{-0.09}}
\expandafter\gdef\csname R@s1.ho.brats.V7C1.mean\endcsname{83.15}
\expandafter\gdef\csname R@s1.ho.brats.V7C1.n\endcsname{3}
\expandafter\gdef\csname R@s1.ho.brats.V7C1.s0\endcsname{83.12}
\expandafter\gdef\csname R@s1.ho.brats.V7C1.s1\endcsname{83.39}
\expandafter\gdef\csname R@s1.ho.brats.V7C1.s2\endcsname{82.93}
\expandafter\gdef\csname R@s1.ho.brats.base.mean\endcsname{83.23}
\expandafter\gdef\csname R@s1.ho.brats.base.n\endcsname{3}
\expandafter\gdef\csname R@s1.ho.brats.base.s0\endcsname{82.98}
\expandafter\gdef\csname R@s1.ho.brats.base.s1\endcsname{83.29}
\expandafter\gdef\csname R@s1.ho.brats.base.s2\endcsname{83.44}
\expandafter\gdef\csname R@s1.ho.btcv.L1.d\endcsname{\ensuremath{+0.71}}
\expandafter\gdef\csname R@s1.ho.btcv.L1.mean\endcsname{78.52}
\expandafter\gdef\csname R@s1.ho.btcv.L1.n\endcsname{3}
\expandafter\gdef\csname R@s1.ho.btcv.L1.s0\endcsname{79.24}
\expandafter\gdef\csname R@s1.ho.btcv.L1.s1\endcsname{78.23}
\expandafter\gdef\csname R@s1.ho.btcv.L1.s2\endcsname{78.10}
\expandafter\gdef\csname R@s1.ho.btcv.L3.d\endcsname{\ensuremath{+0.71}}
\expandafter\gdef\csname R@s1.ho.btcv.L3.mean\endcsname{78.53}
\expandafter\gdef\csname R@s1.ho.btcv.L3.n\endcsname{3}
\expandafter\gdef\csname R@s1.ho.btcv.L3.s0\endcsname{77.85}
\expandafter\gdef\csname R@s1.ho.btcv.L3.s1\endcsname{79.74}
\expandafter\gdef\csname R@s1.ho.btcv.L3.s2\endcsname{78.00}
\expandafter\gdef\csname R@s1.ho.btcv.V7A1.d\endcsname{\ensuremath{+0.49}}
\expandafter\gdef\csname R@s1.ho.btcv.V7A1.mean\endcsname{78.30}
\expandafter\gdef\csname R@s1.ho.btcv.V7A1.n\endcsname{3}
\expandafter\gdef\csname R@s1.ho.btcv.V7A1.s0\endcsname{78.43}
\expandafter\gdef\csname R@s1.ho.btcv.V7A1.s1\endcsname{78.26}
\expandafter\gdef\csname R@s1.ho.btcv.V7A1.s2\endcsname{78.22}
\expandafter\gdef\csname R@s1.ho.btcv.V7C1.d\endcsname{\ensuremath{-0.32}}
\expandafter\gdef\csname R@s1.ho.btcv.V7C1.mean\endcsname{77.50}
\expandafter\gdef\csname R@s1.ho.btcv.V7C1.n\endcsname{3}
\expandafter\gdef\csname R@s1.ho.btcv.V7C1.s0\endcsname{77.67}
\expandafter\gdef\csname R@s1.ho.btcv.V7C1.s1\endcsname{77.29}
\expandafter\gdef\csname R@s1.ho.btcv.V7C1.s2\endcsname{77.54}
\expandafter\gdef\csname R@s1.ho.btcv.base.mean\endcsname{77.82}
\expandafter\gdef\csname R@s1.ho.btcv.base.n\endcsname{3}
\expandafter\gdef\csname R@s1.ho.btcv.base.s0\endcsname{77.57}
\expandafter\gdef\csname R@s1.ho.btcv.base.s1\endcsname{78.15}
\expandafter\gdef\csname R@s1.ho.btcv.base.s2\endcsname{77.73}
\expandafter\gdef\csname R@s1.ho.lits.L1.d\endcsname{\ensuremath{+1.13}}
\expandafter\gdef\csname R@s1.ho.lits.L1.mean\endcsname{81.93}
\expandafter\gdef\csname R@s1.ho.lits.L1.n\endcsname{3}
\expandafter\gdef\csname R@s1.ho.lits.L1.s0\endcsname{81.80}
\expandafter\gdef\csname R@s1.ho.lits.L1.s1\endcsname{81.76}
\expandafter\gdef\csname R@s1.ho.lits.L1.s2\endcsname{82.22}
\expandafter\gdef\csname R@s1.ho.lits.L3.d\endcsname{\ensuremath{+0.50}}
\expandafter\gdef\csname R@s1.ho.lits.L3.mean\endcsname{81.29}
\expandafter\gdef\csname R@s1.ho.lits.L3.n\endcsname{3}
\expandafter\gdef\csname R@s1.ho.lits.L3.s0\endcsname{80.80}
\expandafter\gdef\csname R@s1.ho.lits.L3.s1\endcsname{82.17}
\expandafter\gdef\csname R@s1.ho.lits.L3.s2\endcsname{80.90}
\expandafter\gdef\csname R@s1.ho.lits.V7A1.d\endcsname{\ensuremath{+1.65}}
\expandafter\gdef\csname R@s1.ho.lits.V7A1.mean\endcsname{82.44}
\expandafter\gdef\csname R@s1.ho.lits.V7A1.n\endcsname{3}
\expandafter\gdef\csname R@s1.ho.lits.V7A1.s0\endcsname{81.83}
\expandafter\gdef\csname R@s1.ho.lits.V7A1.s1\endcsname{84.16}
\expandafter\gdef\csname R@s1.ho.lits.V7A1.s2\endcsname{81.34}
\expandafter\gdef\csname R@s1.ho.lits.V7C1.d\endcsname{\ensuremath{+0.85}}
\expandafter\gdef\csname R@s1.ho.lits.V7C1.mean\endcsname{81.65}
\expandafter\gdef\csname R@s1.ho.lits.V7C1.n\endcsname{3}
\expandafter\gdef\csname R@s1.ho.lits.V7C1.s0\endcsname{79.54}
\expandafter\gdef\csname R@s1.ho.lits.V7C1.s1\endcsname{82.76}
\expandafter\gdef\csname R@s1.ho.lits.V7C1.s2\endcsname{82.65}
\expandafter\gdef\csname R@s1.ho.lits.base.mean\endcsname{80.79}
\expandafter\gdef\csname R@s1.ho.lits.base.n\endcsname{3}
\expandafter\gdef\csname R@s1.ho.lits.base.s0\endcsname{79.86}
\expandafter\gdef\csname R@s1.ho.lits.base.s1\endcsname{79.98}
\expandafter\gdef\csname R@s1.ho.lits.base.s2\endcsname{82.54}
\expandafter\gdef\csname R@s1.mirror.amos.L1\endcsname{\ensuremath{+0.48}}
\expandafter\gdef\csname R@s1.mirror.amos.L3\endcsname{\ensuremath{+0.45}}
\expandafter\gdef\csname R@s1.mirror.amos.base\endcsname{\ensuremath{+0.48}}
\expandafter\gdef\csname R@s1.mirror.kits.L1\endcsname{\ensuremath{+0.87}}
\expandafter\gdef\csname R@s1.mirror.kits.L3\endcsname{\ensuremath{+1.41}}
\expandafter\gdef\csname R@s1.mirror.kits.base\endcsname{\ensuremath{+1.52}}
\expandafter\gdef\csname R@s1.nval.acdc\endcsname{40}
\expandafter\gdef\csname R@s1.nval.amos\endcsname{40}
\expandafter\gdef\csname R@s1.nval.brats\endcsname{97}
\expandafter\gdef\csname R@s1.nval.btcv\endcsname{6}
\expandafter\gdef\csname R@s1.nval.kits\endcsname{98}
\expandafter\gdef\csname R@s1.nval.lits\endcsname{27}
\expandafter\gdef\csname R@s1.plan.kits.widths\endcsname{32, 64, 128, 256, 320, 320}
\expandafter\gdef\csname R@s1.rs.07.amos.d\endcsname{\ensuremath{+0.82}}
\expandafter\gdef\csname R@s1.rs.08.amos.d\endcsname{\ensuremath{+0.20}}
\expandafter\gdef\csname R@s1.rs.13.amos.d\endcsname{\ensuremath{-0.97}}
\expandafter\gdef\csname R@s1.rs.15.amos.d\endcsname{\ensuremath{-0.22}}
\expandafter\gdef\csname R@s1.rs.23.amos.d\endcsname{\ensuremath{-0.42}}
\expandafter\gdef\csname R@s1.sp.1.amos.d\endcsname{\ensuremath{+0.51}}
\expandafter\gdef\csname R@s1.sp.2.amos.d\endcsname{\ensuremath{+0.77}}
\expandafter\gdef\csname R@s1.stage.C1\endcsname{replicated}
\expandafter\gdef\csname R@s1.stage.D1\endcsname{replicated}
\expandafter\gdef\csname R@s1.stage.D2\endcsname{cross-validated}
\expandafter\gdef\csname R@s1.stage.L2\endcsname{replicated}
\expandafter\gdef\csname R@s1.stage.L3\endcsname{held-out}
\expandafter\gdef\csname R@s1.stage.L4\endcsname{replicated}
\expandafter\gdef\csname R@s1.stage.L6\endcsname{replicated}
\expandafter\gdef\csname R@s1.stage.N1\endcsname{screened}
\expandafter\gdef\csname R@s1.stage.S2\endcsname{replicated}
\expandafter\gdef\csname R@s1.stage.V5A5\endcsname{replicated}
\expandafter\gdef\csname R@s1.stage.V5B1\endcsname{cross-validated}
\expandafter\gdef\csname R@s1.stage.V5B2\endcsname{cross-validated}
\expandafter\gdef\csname R@s1.stage.V6A1r\endcsname{cross-validated}
\expandafter\gdef\csname R@s1.stage.V7A1\endcsname{held-out}
\expandafter\gdef\csname R@s1.stage.V7A2\endcsname{cross-validated}
\expandafter\gdef\csname R@s1.stage.V7B1\endcsname{replicated}
\expandafter\gdef\csname R@s1.stage.V7B2\endcsname{replicated}
\expandafter\gdef\csname R@s1.stage.V7C1\endcsname{held-out}
\expandafter\gdef\csname R@s1.stage.V8A1\endcsname{replicated}
\expandafter\gdef\csname R@s1.stage.V8A2\endcsname{replicated}
\expandafter\gdef\csname R@s1.stage.V8B1\endcsname{replicated}
\expandafter\gdef\csname R@s1.stage.V8B2\endcsname{cross-validated}
\expandafter\gdef\csname R@s1.stage.W1\endcsname{screened}
\expandafter\gdef\csname R@s1.stage.W2\endcsname{screened}
\expandafter\gdef\csname R@s1.stage.W3\endcsname{screened}
\expandafter\gdef\csname R@s1.stage.n.all\endcsname{25}
\expandafter\gdef\csname R@s1.stage.n.cross-validated\endcsname{6}
\expandafter\gdef\csname R@s1.stage.n.cvplus\endcsname{9}
\expandafter\gdef\csname R@s1.stage.n.held-out\endcsname{3}
\expandafter\gdef\csname R@s1.stage.n.replicated\endcsname{12}
\expandafter\gdef\csname R@s1.stage.n.screened\endcsname{4}
\expandafter\gdef\csname R@s1.tta.acdc\endcsname{with mirroring}
\expandafter\gdef\csname R@s1.tta.amos\endcsname{without test-time augmentation}
\expandafter\gdef\csname R@s1.tta.brats\endcsname{without test-time augmentation}
\expandafter\gdef\csname R@s1.tta.btcv\endcsname{without test-time augmentation}
\expandafter\gdef\csname R@s1.tta.kits\endcsname{without test-time augmentation}
\expandafter\gdef\csname R@s1.tta.lits\endcsname{without test-time augmentation}
\makeatother
